# Supplementary material for: How Good Is NLP? A Sober Look at NLP Tasks through the Lens of Social Impact
Source: arXiv:2106.02359 source file (2023-01-18)
Supplement: Supplementary file 1 [file additional_material.tex]

\section{Moral Philosophy}
\subsection{Intuitional moral philosophy: A practical guide}\label{appd:moral_intuition}
\subsection{Judging by intuitions and commonsense}\label{sec:moral_intuition}
\begin{figure*}[t]
    \centering
    \includegraphics[width=\textwidth]{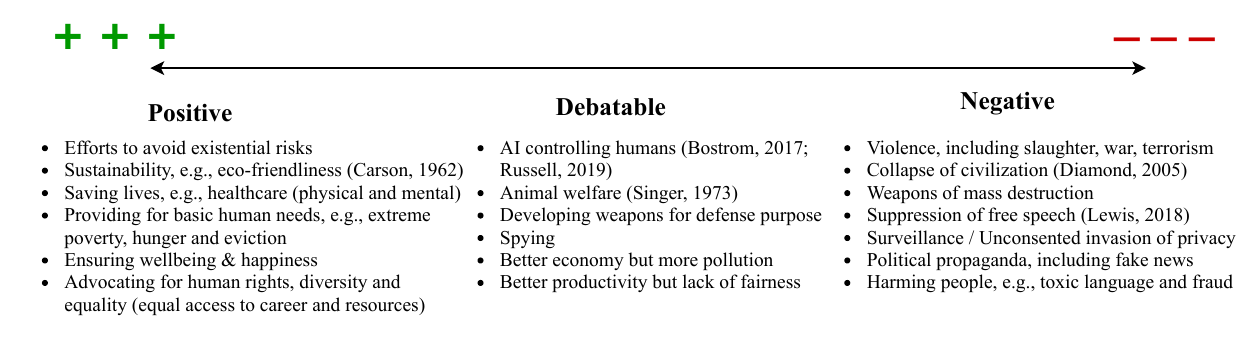}
    \caption{The spectrum from mostly agreed socially good areas (right), to debatable middle areas (center), and mostly agreed socially harmful areas (left). \textcolor{blue}{We will find citations for this list.}}
    \label{fig:commonsense}
\end{figure*}

Before diving into philosophical theories, we make use of intuitionism as one of the mainstream methodologies to moral philosophy \citet{sidgwick1874methods}, and  motivate by intuitions and commonsense moral laws.
%Many people consider intuition provides an a priori epistemological foundation (Poincaré; Brouwer; Dummett; Heyting; Kleene), and
% moral laws as self-evident, just as in Immanuel Kant once wrote, ``the starry heavens above me and the moral law within me.''
%\citet{sidgwick1874methods} formally lists intuitionism as one of the mainstream methodologies to moral philosophy. It is also a common methodology to use thought experiments with intuitive judgements to test philosophical theories. Moreover, commonly shared strong intuitions can tie and unite a society of people even without academic backgrounds. 

We can understand the intuitional moral judgements from the light of universal values, the set of values that are agreed by most people in society across a great diversity of human cultures \cite{Schwartz-todo}. The common universal values include survival of the human species \cite{dawkins1976selfish,ord2020precipice}, pleasure \cite{veenhoven2003hedonism}, democracy \cite{sen1999democracy}, non-violence \cite{gandhi1942non}, and sustainability \cite{goodland1996environmental}. For example, aversion to wars and mass killing can be attributed to non-violence, and the instinct to keep our mankind as a species to last. The pursuit towards happiness and well-being can be attributed to the universal pursuit of pleasure, which develops into moral philosophy streams such as utilitarianism and egoism, which will be introduced in the next subsection.

In Figure~\ref{fig:commonsense}, we present a spectrum from acts with mostly-agreed upon positive social impact  or negative social impact, as well as examples of several debatable areas. More detailed rationale behind the directions listed in the spectrum is discussed in Appendix~\ref{appd:moral_intuition}.

%\paragraph{Interpretation by universal values.}

Many people consider the moral law as self-evident, just as in Immanuel Kant once wrote, ``the starry heavens above me and the moral law within me.'' 
\citet{sidgwick1874methods} formally lists intuitionism as one of the mainstream methodologies to moral philosophy. Intuitions are useful because they are the grounds before theorizing, which explains why thought experiments with intuitive judgements are used as a common methodology to test philosophical theories. Moreover, commonly shared strong intuitions can tie and unite a society of people even without academic backgrounds. In the following, we will list some socially good and bad directions that receive large consensus, and then some typical debatable acts. 

\paragraph{Good for certain}
\begin{itemize}[nolistsep]
    \item Efforts to avoid existential risks
    \item Sustainability, including eco-friendly activities \cite{carson1962silent}
    \item Saving lives, including healthcare (physical and mental health)
    \item Providing for basic human needs, including the fight against extreme poverty, hunger and eviction
    % \item Enlightenment, incl. 9-12 years of schooling 
    \item Ensuring well-being \& happiness
    \item Advocating for human rights,  diversity and equality (equal access to career and resources)
\end{itemize}

\paragraph{Bad for certain}
\begin{itemize}[nolistsep]
    \item Violence, including slaughter, war, terrorism
    \item Collapse of civilization \cite{diamond2005collapse}
    \item Weapons of mass destruction %(north korea disagrees)
    \item Suppression of free speech \cite{lewis2008freedom}
    \item Surveillance / Unconsented invasion of privacy (controversial, cases of apple giving data to FBI; tradeoff between tracking and criminals)
    \item Political propaganda, including fake news
    \item Harming people, including toxic language and fraud
\end{itemize}

\paragraph{Debateable}
\begin{itemize}[nolistsep]
    \item AI controlling humans \cite{bostrom2017superintelligence,russell2019human}
    \item Animal welfare \cite{singer1973animal}
    \item Developing weapons for defense purpose
    \item Spying
    \item Better economy but more pollution
    \item Better productivity (accuracy) but lack of fairness
\end{itemize}

\paragraph{Interpretation from Universal Values.}

\textcolor{red}{MS: I am not sure if we need to spend so much space on the rationales since the list above seems self-explanatory}

\paragraph{Rationale.}
Now we explain some of the rationales behind the list of social good, bad, and debateable areas. Among the \textbf{social good acts}, the most important one is the \textit{efforts to avoid existential risks}. Existential risks are the catastrophic risks that can permantently curtail the potential of humanity \cite{bostrom2002existential}, including natural disasters such as a 1-km-wide asteroid hitting the earth, supervolcanoes, or man-made disasters such as a nuclear war, and genetically engineered deadly virus \cite{sandberg2008global,ord2020precipice}. We want to avoid existential risks due to our instinct as a species, and we want our genes to last as long as possible \cite{dawkins1976selfish}.
Apart from disruptive existential risks, we also want to avoid consumption curves that are monotonically increasing; instead, we promote \textit{sustainability} such as eco-friendly acts. The remaining five directions of social good are shared by human nature, and corresponding more or less to Maslow's hierarchy of needs from physiological needs, and safety needs, to self-actualization \cite{maslow1943theory}. We want to help all humans -- first saving lives, then satisfying basic human needs such as hunger, and moreover, some higher pursuits such as enlightenment by education, happiness, and protection of human rights, diversity, and equality.

Among the \textbf{socially harmful acts}, it is commonly not accepted to resort to violence for the purpose of resource redistribution. Indirect leads to violence is also unacceptable such as developing weapons for mass destruction. Other acts such as suppression of free speech, surveilance, propaganda, and delibrate harms such as toxic language are also commonly recognized as harmful.

Regardless of the consensus on many socially good and bad acts, there are a large amount of areas that remain \textbf{debateable}, such as the fear of AI controlling humans, which is common in the public reception of AI through news and some overclaiming literature. It is debateable because if we define the research of AI as harmful, then our academic conferences would not take place, and AI researchers will look for other jobs. We continue in the field of AI because we believe that there is more hope than desperation that AI can bring a more productive, better future of human society. There are also other debateable areas such as doing one good at the sacrifice of another thing, such as increasing economy at the cost of environment, or developing self-driving that causes drivers to first lose jobs and afterwards a tough transition to look for other careers.
\subsection{Sidgwick and Parfit's Perspectives}
We introduce below six philosophical perspectives to judge moral laws, based on \citet{sidgwick1874methods} (the first three) and \citet{parfit2011matters} (the last three).
\begin{enumerate}[nolistsep]
    \item Intuitionism: judging by intuitive morality
    \item Egoism: maximizing the happiness of oneself
    \item Utilitarianism: maximizing the happiness of all sentient beings
    \item Kantian deontology: judging by a set of rules and duties instead of consequences
    \item Consequentialism: judging by the ultimate consequences of one's conduct
    \item Contractualism: following the social contract \cite{rousseau1762social} that individuals surrender some freedoms in exchange for protection of their remaining rights or maintenance of the social order.
\end{enumerate}
% Note that utilitarianism seeks for the optimal course of act according to impartial concerns for the pleasures and pains for all sentient beings \cite{sidgwick1874methods}. Peter Singer extends the utilitarianism to sentient animals \cite{singer1973animal}, corresponding to the wave of animal welfare which results in laws and regulations in the US and Europe \cite{matheny2007farm,veissier2008european}.
\paragraph{A radar diagram.}
The six perspectives provides us dimensions to think about the impact $I(a)$ of an act $a$, so that the final decision is more reliable than one single subjective thought.

Although no measurement criteria are available, for institutional decision-making, it can be a good heuristics to use radar diagrams.
For an unwritten (mental) rating about an act $a$ by $(r_1, r_2, \dots, r_6)$ where $r_i$ is the rating on the $i$-th theory, We can draw a radar diagram to facilitate our judgements. For example, when we try to decompose our reasoning for why economic development is generally good, we can use Figure~\ref{fig:radar} to show that by our ``unwritten evaluations,'' economic development scores high on all dimensions. 
\begin{figure}[h]
    \centering
    \includegraphics[width=0.9\columnwidth]{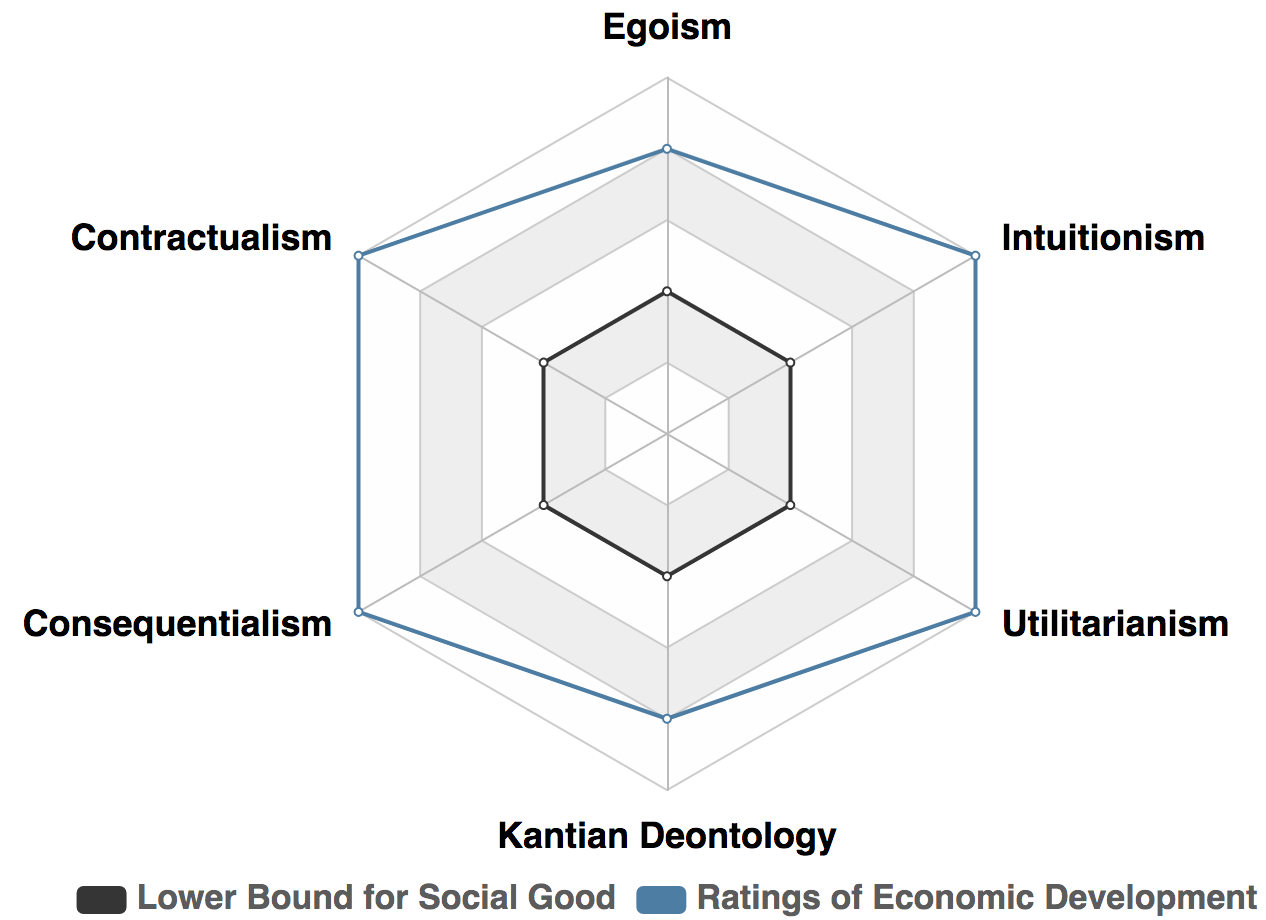}
    \caption{(Estimated) Ratings of economic development by all six philosophies.}
    \label{fig:radar}
\end{figure}
% Made by https://online.visual-paradigm.com/app/diagrams/#diagram:proj=0&type=RadarChart&gallery=/repository/316147c6-cc9b-4e75-aae7-740f8229028f.xml&name=Employee%20Skill%20Analysis
% https://online.visual-paradigm.com/drive/#diagramlist:proj=0&new=RadarChart
\paragraph{Towards a unified theory.}
Other moral uncertainty theories: \url{https://concepts.effectivealtruism.org/concepts/moral-uncertainty/}

A relentless effort in science is to find unification of different theories. Although this can be what philosophers have worked on for centuries and millennia, here we present a tentative sketch to use three principles to unify the above six perspectives:

(1) Just like the example of solving global poverty, hypothetically there exist optimal, harmonious, oracle moral laws, which can achieve a good score by most perspectives. For example, \citet{sidgwick1874methods} states that intuitionism and utilitarianism can in essence be harmonious with each other.

(2) At suboptimal points, sometimes there are tradeoffs between one dimension and another, such as egoism and utilitarianism -- if the total utilitarianism has to sacrifice somebody, then if that person is unwilling, their egoism is harmed.

(3) When judging social good of an act, we also want this act to not score extremely bad on any perspective, according to the moral uncertainty theory which maximizes expected choiceworthiness \missingcite{}. The more balanced scores an act has, the more robust the moral judgement is.
% want it to pass a basic score on all six perspectives, in order to prevent extreme and biased use of one perspective, such as killing a child for the good of a group of people by consequentialism. To prevent these cases, the moral uncertainty theory maximizes expected choiceworthiness, which requires that each act to have as much balanced score by different criteria as possible. The more balanced, the more morally robust a solution is.
Similarly, \citet{parfit2011matters} fuses the last three ethical theories by the comment that they ``climb the same mountain on different sides.'' Specifically, he makes the Triple Theory to judge the rightness and wrongness of an act by whether it is disallowed by the principles that are optimific (i.e., Consequentialisim), uniquely universally willable (i.e., Kantianism), and not reasonably rejectable (i.e., Contractualism). 
% “an act is wrong just when such acts are disallowed by some principle that is optimific, uniquely universally willable, and not reasonably rejectable.” (Vol. I, p.413)

% \textcolor{red}{MS: So what does this theory say about NLP or AI more broadly? How do I apply this?}
% \textcolor{blue}{Zhijing: We will use the theory in Section~\ref{sec:nlp_examples}.}

\subsection{Principles (Optional content; will be cut for page limit)}
(0) Do no harm principle
(1) Universalizability principle
% Test a moral law by whether it works of any number of people do it 
\cite{parfit2011matters}

\noindent
(2) Interpersonal addition theorem \cite{broome2017weighing}
\subsection{Thought experiments as a thinking tool.} 
Section 2 to 4 provide a general framework to judge and evaluate NLP for social good. However, due to the complexity in real world scenarios, there is no clear formula to put every variable into consideration and generate a 100\% certain answer. Nonetheless, our paper aims to provide practical insights, so we will propose several simplified, ideal scenarios for thought experiments, and deduct the priority research directions of NLP under such scenarios.

\paragraph{If 99\% of the population are starving.}
The first scenario we assume is the extreme lack of food on earth. Food resources is the basic needs of human beings. Most civilizations do not have enough food for everyone for a long historical period, and even in the contemporary era, XX\% are starving every day. If it happens that the food on earth can only feed 1\% of the population, and leave the rest 99\% in starvation, then the priority task is to use technology on agricultural production. For example, we can use NLP for a Question and Answer system so that people who want to do research on food production can easily get the answer from an existing database. We can also use NLP to power a summarization system, so that researchers do not need to read through thousands of papers but instead have a quick summary of the previous research progress. There can also be an NLP to automatically generate public news, tweets, or forums so that the emotions of the starving people can be addressed, while the scientists are looking for solutions.

\paragraph{When is Green NLP useful?}
Another interesting topic is the green NLP track that this year's NAACL 2021 newly proposed. Green NLP promotes NLP research to consume less energy (e.g., GPU computational power). There are some cases that this direction is crucially important, and there can also be some other cases where this direction is not necessarily correct. The essence of the problem is a tradeoff between resource usage and scientific progress. A simplified analogy is that every human consumes some resources for essential activities like eating, although it is true that if the person's basic needs are met, then they should save resources for sustainability. However, we cannot starve the person by giving them an overly-stringent resource budget. Similiarly for green NLP, the main purpose of NLP research is to make scientific progress, and if some research groups (e.g., OpenAI) do think that running a lot of GPU hours is worth in exchange for the scientific progress, then with enough justification, such resource consumption can be considered as reasonable. But if to achieve the same scientific progress, we can choose between a smaller resource consumption and a larger consumption, definitely we should opt for the smaller one. Or another scenario when green NLP is very important is when, for example, the earth will have a runaway climate change if the temperature rises for 0.00001 more degree, then we should immediately stop NLP experiments that emit carbon dioxide. In summary, the actual choice between green NLP and faster scientific progress depends on case-by-case judgements, although it is generally a valuable concept to bring up to the community.

\paragraph{Several other thought experiments.}

\section{Priority estimation}

\textcolor{blue}{The following two topics can be mentioned, optionally, according to space limit.}
\paragraph{Imperfect information problem.}

\paragraph{Online algorithm (active learning).}

% \subsection{What priority causes have been identified?}
% Different organizations rank priorities differently, and here we will list examples of several organizations.

% \paragraph{Goals by United Nations.}
% The United Nations (UN) has set a list of goals:\footnote{\url{https://sdgs.un.org/goals}}
% \begin{enumerate}[nolistsep]
%     \item No poverty
%     \item Zero hunger
%     \item Good health and well-being
%     \item Quality education
%     \item Gender equality
% \end{enumerate}
% \paragraph{Effective Altruism.}
% Effective Altruism is a newly emerged philosophy with lots of community engagement from academia, industry, and philanthropy organizations. 
% It aims to establish a new philosophy for the pursuit of good what the Enlightenment did for the pursuit of truth. It
\paragraph{Global Priority Research.}
The field of global priority research uses three pillars to judge the most urgent global problems to work on: scale (how many are affected by the problem), neglectedness (how many people are working on it already), solvability (how easy it is to make progress), and personal fit. These are adopted by organizations such as Open Philanthropy Project, and Future of Human Institute at Oxford University.
The current priority list that global priority researchers establish for effective social good includes global health and development, farm animal welfare, and reduction of existential risks (particularly including AI safety). 
% % \paragraph{Distribution of Money.}
% % We start with the distribution of money in terms of general directions. (Hopefully there can be some resources for these numbers on NLP fundings?)

% % The money distribution for some major cause areas are below:
% % \begin{table}[h] 
% % \small
% %     \centering
% %     \begin{tabular}{ll}
% %     \toprule
% %      Cause & Annual Spending (USD) \\ \midrule
% %      Global R\&D & 1.5 trillion \cite{unesco2017facts} \\
% %      Luxury Goods & 1.3 trillion \cite{d2015luxury} \\
% %      US Social Welfare & 900 billion \cite{ferrara2011america} \\
% %      Climate Change & $>$300 billion \cite{buchner2014global} \\
% %      Global Poverty & $>$250 billion\footnote{\url{https://80000hours.org/problem-profiles/health-in-poor-countries/}} \\
% %      Nuclear Security & 1-10 billion\footnote{\url{https://80000hours.org/problem-profiles/nuclear-security/}} \\
% %      Pandemic Prevention & 1 billion\footnote{\url{https://80000hours.org/problem-profiles/biosecurity/}} \\
% %      AI Safety Research & 10 million\footnote{\url{https://80000hours.org/problem-profiles/positively-shaping-artificial-intelligence/}} \\
% %      \bottomrule
% %     \end{tabular}
% %     \caption{Caption}
% %     \label{tab:my_label}
% % \end{table}

% % The clear discrepancy reflected by the above table is the (probably misguided) trend to improve our well-being by luxury goods. Astoundingly, the expenditure on luxury goods is about four times the investment to prevent climate change, and the money given to help the poor people.

% % If you look at political attention, you’d find a similar picture to the funding figures. An overwhelming amount of political attention goes on concrete issues that help the present generation in the short-term, since that’s what gets votes. Catastrophic long-term risks are far more neglected.

\section{Applying the theories}
\paragraph{Estimating the sign of $I(t)$ for a Stage-4 technology $t$.} We first apply the discussions in \cref{sec:philosophy} to provide basic estimation of impact for Stage-4 technologies in three categories:

(1) Commonsense positive NLP: NLP for agriculture (to help hunger), NLP for healthcare, NLP for education, and NLP for low-resource languages of underdeveloped countries (to help equality).

(2) Commonsense negative NLP: NLP for propanganda or mind control, NLP for fraud, etc.

(3) Judging controversial uses of NLP by six philosophical theories: 
GreenNLP (=tradeoff between higher accuracy and more energy cost), NLP to replace human labor (=higher productivity but some people lose jobs), NLP for selection process (=more efficiency but might induce bias). We reject directions if they are extremely bad by one of the six philosophical criteria according to moral uncertainty theory. If some are still controversial, we resort the decision to social science studies or wait for more statistical analyses after some test usages.

\paragraph{More accurate estimation of $I(t)$ for a Stage-4 technology $t$.}
If the end impact can be decomposed to several use cases with more certain social impact estimation, we can obtain the final impact of the technology by aggregating the impact of all use cases by corresponding quantities. Taking the example of the text style transfer application between male and female writings, its use cases are double-edged swords: user identity obfuscation (for better privacy) and easier online fraud (e.g., for a male to pretend as a female) \cite[example taken from ][]{jin2020deep}. So if we aggregate its impact $I(t)$ by Eq~\eqref{eq:impact_stage5}, the end impact of this technology is almost neutralized. 

\paragraph{Using causal model to estimate $I(t)$ for technology $t$ in Stage 1, 2, and 3.}

Apart from Stage-4 technologies whose end impact can be approximated by Eq.~\eqref{eq:impact_stage5}, there are lots of NLP research in Stage 1, 2, and 3, which will need in addition the guide of Eq.~\eqref{eq:impact_indirect} to calculate their indirect cause for potential end impacts. For example, the pretrained model BERT \cite{devlin-etal-2019-bert} does not directly interact with use cases, but it boosts the performance of many other NLP technologies such as machine translation, summarization, dialog generation, and so on. The final impact of BERT is generally positive if the sum of end impacts of these technologies improved by BERT is positive. On the potential negative side, if an upstream technology is more likely to be used to downstream applications to generate propaganda or mind control, then this technology's expected impact will be negative.

We provide some preliminary discussions of the impact of several popular NLP tasks in \cref{sec:nlp_example_impact}.

\section{Examples of 4 Stages}
\begin{table*}[t]
    \small
    \centering
    \begin{tabular}{p{0.2\textwidth}p{0.2\textwidth}p{0.2\textwidth}p{0.2\textwidth}}
    \toprule
    Stage 1 & Stage 2 & Stage 3 & Stage 4 \\ \hline
    \begin{itemize}[nolistsep,leftmargin=0in]
        
        \item Psycholinguistics
        \item Model development principles
        \item NLP field analysis
        \item Emergent languages
    \end{itemize}
    &
    Traditional NLP
    \begin{itemize}[nolistsep,leftmargin=0in]
        \item syntax parsing
        \item syntax-based generation
        \item segmentation
        \item phonology
        \item morphology
        \item text normalization
        \item word meaning
        \item noun ontology
        \item language grounding
        \item word order
        \item tagging
        \item coreference
    \end{itemize}
    Basic NLP tasks
    \begin{itemize}[nolistsep,leftmargin=0in]
        \item language modeling
        \item topic modeling
        \item semantic parsing
        \item knowledge graph
        \item 

    \end{itemize}
    
    Social-Good
    \begin{itemize}[nolistsep,leftmargin=0in]
        \item Interpretability
        \item Robustness
        \item Better out-of-distribution prediction
        \item Bias
    \end{itemize}
    
    Others
    \begin{itemize}[nolistsep,leftmargin=0in]
        \item Dataset
        \item Evaluation metrics
        \item Model architecture
        \item Greener models
    \end{itemize}
    &
    Social-Good
    \begin{itemize}[nolistsep,leftmargin=0in]
        \item Low-resource applications
    \end{itemize}
    Applications
    \begin{itemize}[nolistsep,leftmargin=0in]
        \item sentiment and argument analysis
        \item Intent classification
        \item information extraction
        \item information retrieval
    \end{itemize}
    \begin{itemize}[nolistsep,leftmargin=0in]
        \item dialog, QA, interactive system
        \item speech
        \item machine translation
        \item summarization
        \item data-to-text generation
        \item Code generation
        \item caption generation
        \item style transfer
        \item grammatical error correction
        \item automatic grading
        \item special text generation (pun, sarcasm, suspense)
    \end{itemize}
    
    & 
    Application to other domains
    \begin{itemize}[nolistsep,leftmargin=0in]
        \item Physical healthcare
        \item Mental healthcare
        \item Education
        \item Legal and political text analysis
        \item Legal judgement
        \item stock market prediction
        \item robotics
        
    \end{itemize}
    
    Media-related
    \begin{itemize}[nolistsep,leftmargin=0in]
        \item Media profiling
        \item Preventing misinformation
    \end{itemize}
    \\ \bottomrule
    \end{tabular}
    \caption{Caption}
    \label{tab:acl_fine_categories}
\end{table*}

Stage-2: information management, information discovery

Deployed products of NLP in stage 4: NLP for disaster response, spell check (Salesforce's contact form spell check), autocomplete (Google search, Gmail, Google doc), search autocorrect (Hubspot), spam filters, smart search = better information retrieval (Google search, Klevu's eCommerce search), machine translation (Lilt), chatbots (Alexa with unlimited Skills, Google Assistants, Siri, Facebook messenger bots), virtual assistants (Mastercard bot, Zendesk's Answer Bot software, chatbot on websites), voice text messaging, 
user feedback analysis (Wonderflow's Wonderboard, IBM SPSS Text Analytics for Surveys)
recommendation systems based on textual record of the user, social media monitoring to discover customer needs (Sprout Social), market strategy-featured writing assistant (MarketMuse)

Every minute, there are 350 million new tweets, 4.4 million Google searches, 78 million wordpress posts, and 294 billion emails (Smart Insight, 2020).\footnote{\url{https://www.smartinsights.com/internet-marketing-statistics/happens-online-60-seconds/}}
